# Supplementary material for: Hot-Carrier Generation in Plasmonic Nanoparticles: The Importance of Atomic Structure
Source: arXiv:2002.12087 ancillary file (2020-07-29)
Supplement: Supplementary file 1 [file Supplementary_Information.pdf]

Supplementary Information

# Hot-Carrier Generation in Plasmonic Nanoparticles: The Importance of Atomic Structure

Tuomas P. Rossi,† Paul Erhart,† and Mikael Kuisma‡

† *Department of Physics, Chalmers University of Technology, SE-412 96 Gothenburg, Sweden*
‡ *Department of Chemistry, Nanoscience Center, University of Jyväskylä, FI-40014 Jyväskylä, Finland*

## Contents

**Supplementary Figures** **2**
S1. Distribution of the stored energy over electron-hole transition energies in $Ag_{561}$ . . . 2
S2. Rate of change in energy stored in $Ag_{561}$ . . . 2
S3. Real-time dynamics in $Ag_{561}$ up to 60 fs . . . 3
S4. Real-time dynamics in $Ag_{55}$ up to 120 fs . . . 3
S5. Energy contributions from real and imaginary parts of density matrix . . . 4
S6. Electron-hole transition contributions to Coulomb energy . . . 4
S7. Photoabsorption spectra and densities of states of silver nanoparticles . . . 5
S8. Hot-carrier distributions in silver nanoparticles . . . 6
S9. Atomic-scale distributions of hot holes in silver nanoparticles . . . 7
S10. Effect of the dynamic response kernel on the results . . . 7

**Supplementary Notes** **8**
S1. Perturbation expansions of time-dependent quantities . . . 8
S2. Energy in terms of real and imaginary parts of density matrix . . . 10
S3. Rate of energy change . . . 11
S4. Practical evaluation of energy and its rate of change . . . 11

**Supplementary References** **11**

# Supplementary Figures

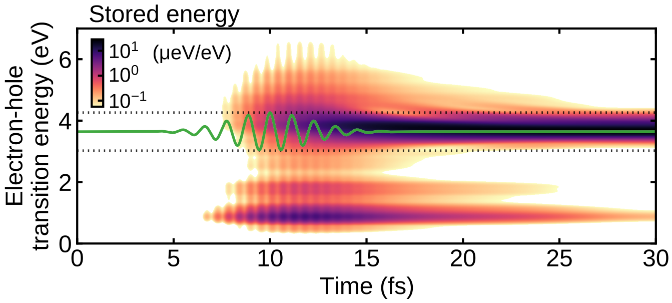


**Supplementary Figure S1: Distribution of the stored energy over electron-hole transition energies in $\mathbf{Ag_{561}}$.** Distribution of the stored energy $E_{ia}(t)$ (Supplementary Note S1) over electron-hole transition energies $\omega_{ia}$, *i.e.*, $E(\omega, t) = \sum_{ia} E_{ia}(t)\delta(\omega - \omega_{ia})$ with a Gaussian smoothing over $\omega$ is shown. The color scale is logarithmic. The pulse is overlaid at its frequency $\omega_0$ and the pulse width $\sigma = \sqrt{2}/\tau_0$ is indicated as dotted lines at $\omega_0 \pm 2\sigma$. The contribution from resonant transitions in Fig. 1e in the main text comprises of transitions with energy $\omega_{ia}$ between $\omega_0 \pm 2\sigma$, and that from the non-resonant transitions comprises of the plasmonic low-energy transitions ($\omega_{ia} < \omega_0 - 2\sigma$) and the screening high-energy transitions ($\omega_{ia} > \omega_0 + 2\sigma$).

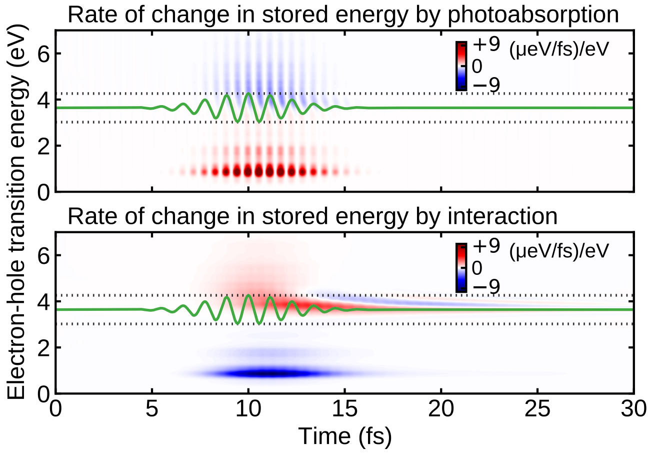


**Supplementary Figure S2: Rate of change in energy stored in $\mathbf{Ag_{561}}$.** Distributions of the rate of change $\dot{E}_{ia}(t)$ over electron-hole transition energies $\omega_{ia}$ divided into photoabsorption and interaction components (Supplementary Note S3). The plasmonic low-energy transitions absorb the energy from the resonant pulse (upper panel) and the energy is subsequently redistributed to higher-energy screening transitions and resonant hot-carrier transitions (lower panel). The screening transitions return their energy back to the field weakening the photoabsorption by plasmon (upper panel), and after the plasmon has dephased, the absorbed energy remains in hot-carrier transitions.

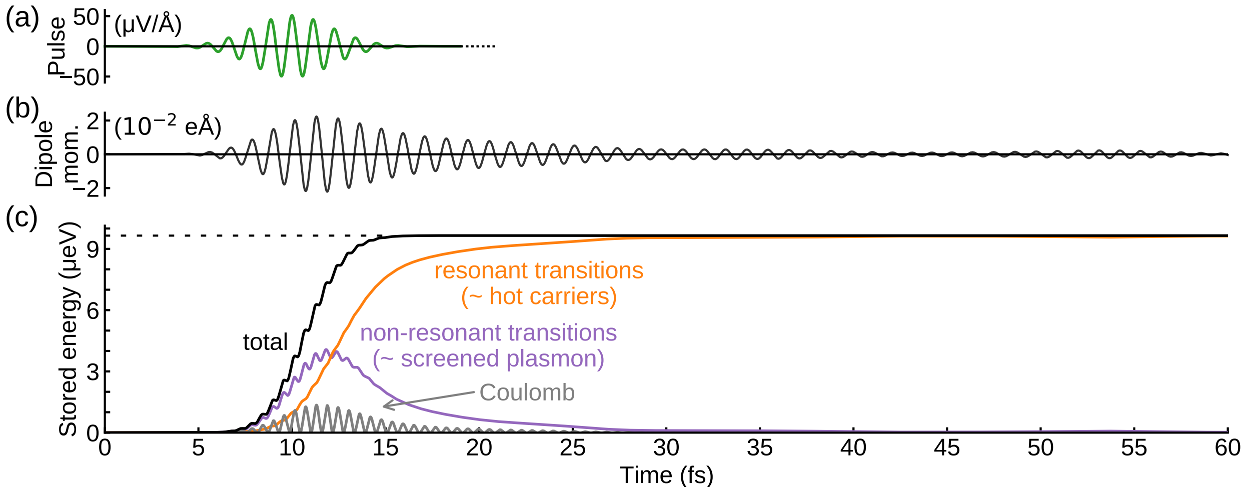


**Supplementary Figure S3: Real-time dynamics in $Ag_{561}$ up to 60 fs.** (a) Electric field pulse impacting the nanoparticle. (b) Time-dependent dipole moment response of the nanoparticle. (c) Time evolution of the energy stored in the excited electronic system divided into non-resonant and resonant contributions as in Fig. 1 in the main text. The plasmon has dephased at 30 fs and only a minor recurrence of the plasmon is visible at around 55 fs.

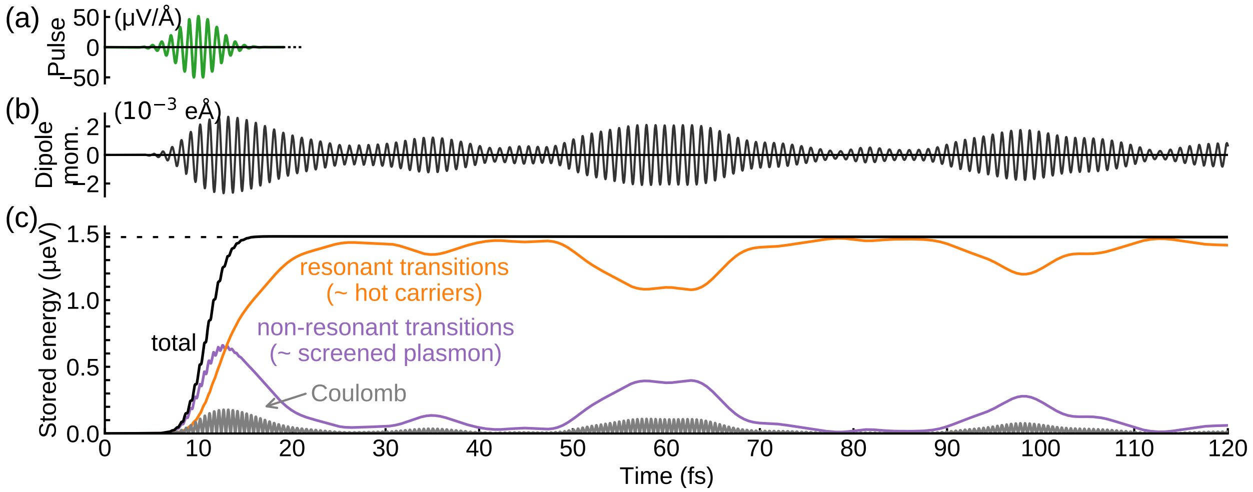


**Supplementary Figure S4: Real-time dynamics in $Ag_{55}$ up to 120 fs.** (a) Electric field pulse impacting the nanoparticle. (c) Time-dependent dipole moment response of the nanoparticle. (e) Time evolution of the energy stored in the excited electronic system divided into non-resonant and resonant contributions analogously to Fig. 1 in the main text. The response of $Ag_{55}$ consists of a few separate resonances instead of a single broad one, which appears in the time-domain as Rabi oscillations and recurrence of the plasmon. At long time scales, the dynamics is expected to be affected by electron–electron interaction and other scattering processes that lead to excitation decay but are not included in the present description.

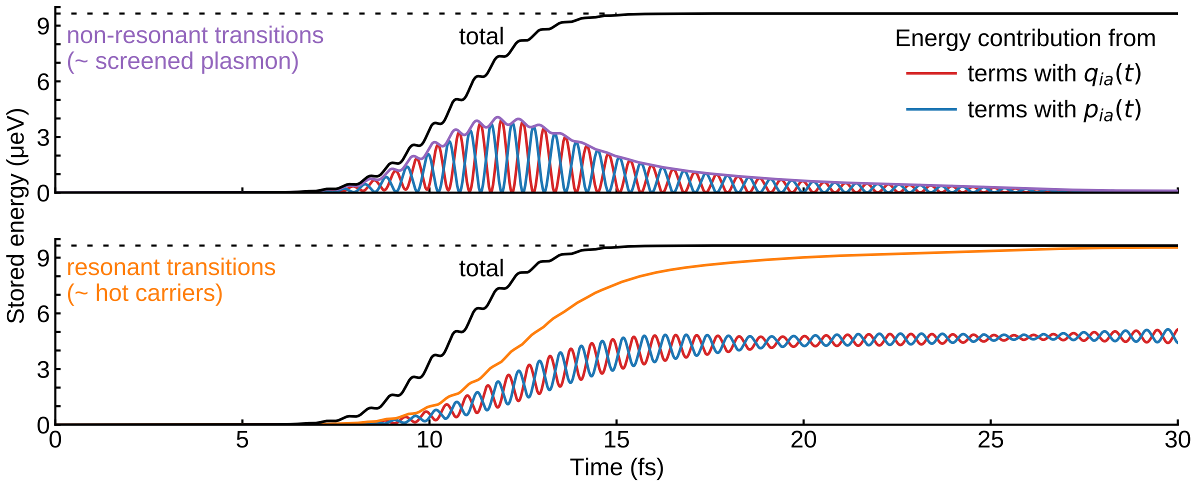


**Supplementary Figure S5: Energy contributions from real and imaginary parts of density matrix.** The energy stored in non-resonant and resonant transitions (Fig. 1 in main text) is further decomposed to contributions from the real and imaginary parts of density matrix, *i.e.*, from $q_{ia}(t)$ and $p_{ia}(t)$ defined in Eq. (33), respectively. Specifically, terms with $q_{ia}(t)$ are $\frac{1}{2}\omega_{ia}q_{ia}^2(t) + \frac{1}{2}q_{ia}(t)\sum_{jb} K_{ia,jb}q_{jb}(t)$ and terms with $p_{ia}(t)$ are $\frac{1}{2}\omega_{ia}p_{ia}^2(t)$, summing up to the energy $E_{ia}(t)$ in Eq. (35). The upper panel illustrates that plasmon can be thought as a classical harmonic oscillator with energy oscillating between density ($q_{ia}$ or "position coordinate") and current ($p_{ia}$ or "momentum coordinate").

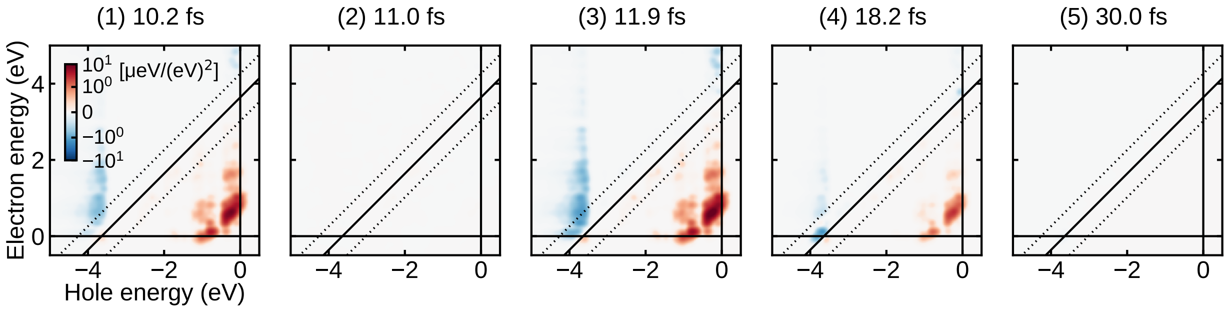


**Supplementary Figure S6: Electron-hole transition contributions to Coulomb energy.** The contributions are visualized as TCM on a logarithmic color scale similarly to the total energy in Fig. 2 in the main text. Note that while the screening high-energy transitions have negative contribution to the Coulomb energy, the total energy contribution from every electron-hole transition is positive as depicted in Fig. 2 in the main text. See Eq. (35) and discussion therein for the energy terms.

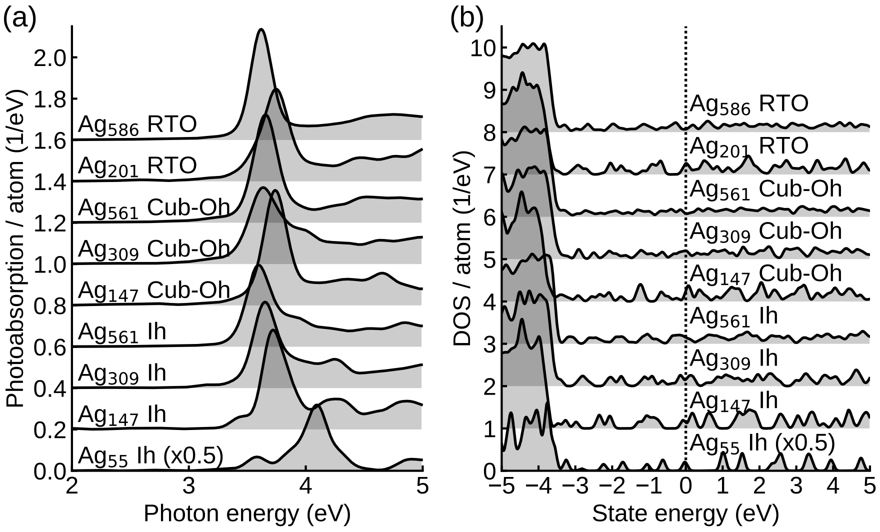


**Supplementary Figure S7: Photoabsorption spectra and densities of states of silver nanoparticles.** (a) Photoabsorption spectra and (b) densities of states (DOS) of silver nanoparticles of icosahedral (Ih), cuboctahedral (Cub-Oh), and regularly truncated octahedral (RTO) shapes. The Fermi level is at 0 eV in panel b. The data for $Ag_{55}$ has been multiplied by 0.5. For each shape, the plasmon resonance show a redshift with increasing particle size, following the shift in the d-band onset with respect to the Fermi level apart from the small $Ag_{55}$. $Ag_{309}$ Cub-Oh is an exception with broader and more redshifted plasmon peak than expected based on $Ag_{147}$ and $Ag_{561}$, with a corresponding difference seen in the d-band onset.

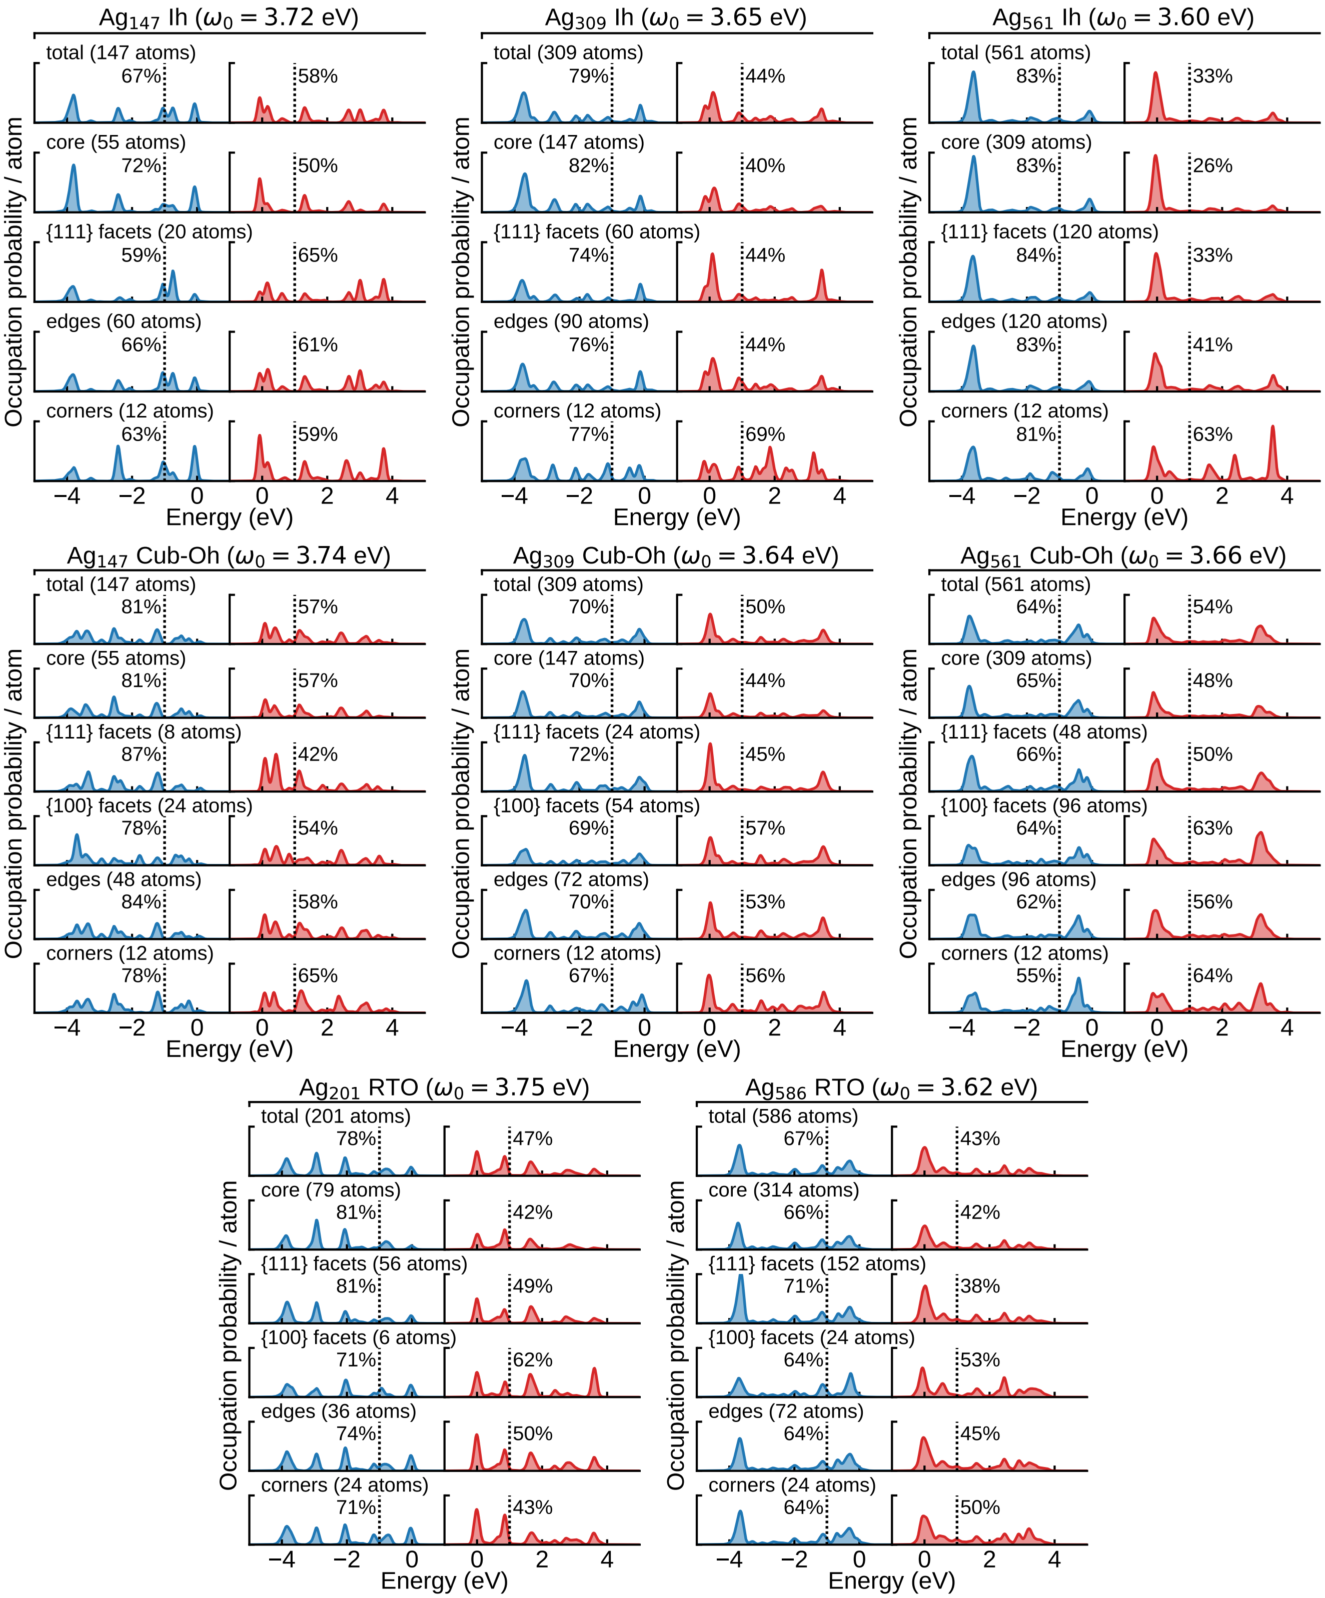


**Supplementary Figure S8: Hot-carrier distributions in silver nanoparticles.** Occupation probabilities of hole and electron states after plasmon decay in silver nanoparticles of icosahedral (Ih), cuboctahedral (Cub-Oh), and regularly truncated octahedral (RTO) shapes. Occupation probabilities at different atomic sites (core, facets, edges, and corners) are also shown. The distributions are per atom (the number of atoms in each set is indicated in parenthesis). The percentages adjacent to the $-1\,\text{eV}$ and $1\,\text{eV}$ dotted lines indicate the amount of holes and electrons with energy $< -1\,\text{eV}$ and $> 1\,\text{eV}$, respectively, in comparison to the total amount in each set. Scale is the same in each plot.

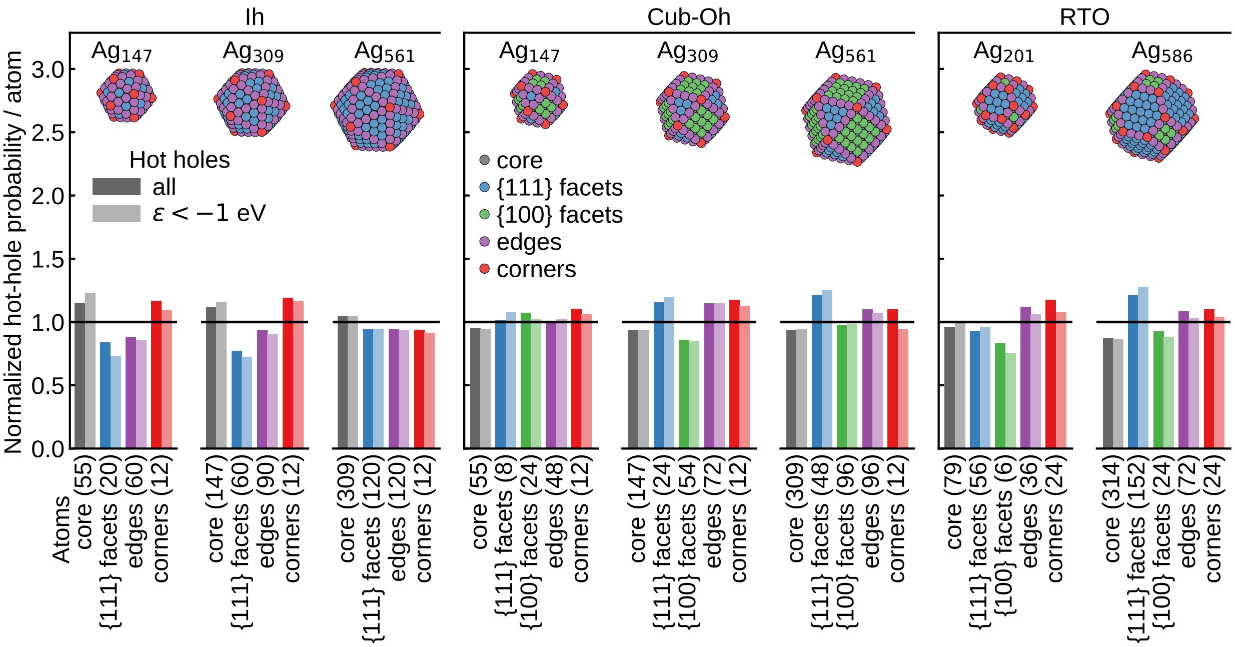


**Supplementary Figure S9: Atomic-scale distributions of hot holes in silver nanoparticles.** Spatial distribution of hot holes generated on different atomic sites in selected nanoparticles. Most distributions show relatively small variations from spatially uniform distribution and no surface or core site appear to be systematically favored. The distribution of hotter holes (energy $\epsilon < -1$ eV) is similar to that of all generated holes due to the d electron states dominating the hot-hole distribution (Supplementary Fig. S8).

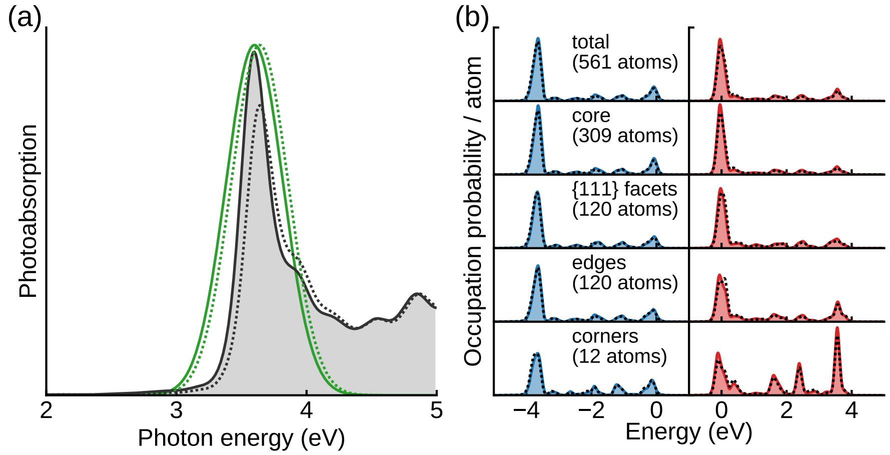


**Supplementary Figure S10: Effect of the dynamic response kernel on the results.** (a) Photoabsorption spectra of $Ag_{561}$ calculated with the adiabatic GLLB-sc exchange-correlation (XC) potential (solid shaded black line) and random-phase approximation (RPA) (dotted black line). The pulse is tuned to the plasmon resonance (3.60 eV for the adiabatic GLLB-sc and 3.64 eV for RPA; solid and dashed green lines, respectively). (b) Hot-carrier distributions in $Ag_{561}$ calculated with the adiabatic GLLB-sc (solid shaded lines) and RPA (dotted lines). The ground state is calculated with GLLB-sc XC potential in all the cases. The differences in the results obtained with different dynamic response kernels are minor.

# Supplementary Notes

**Supplementary Note S1: Perturbation expansions of time-dependent quantities.**

**Wave function.** The expansion of the time-dependent wave function up to second order in perturbation is (notation: $|i(t)\rangle = \psi_i(t)$ and $|i\rangle = \psi_i^{(0)}$)

$$|i(t)\rangle = e^{-i\epsilon_i t}|i\rangle + \sum_j e^{-i\epsilon_j t} C_{ji}^{(1)}(t)\,|j\rangle + \sum_j e^{-i\epsilon_j t} C_{ji}^{(2)}(t)\,|j\rangle\,, \tag{1}$$

which gives the projection $\langle k|i(t)\rangle = e^{-i\epsilon_k t}\left(\delta_{ik} + C_{ki}^{(1)}(t) + C_{ki}^{(2)}(t)\right)$. Consider the norm up to second order

$$\langle j(t)|i(t)\rangle = \sum_k \langle j(t)|k\rangle\langle k|i(t)\rangle = \delta_{ji} + \underbrace{C_{ji}^{(1)}(t) + C_{ij}^{(1)*}(t)}_{=0} + \underbrace{C_{ji}^{(2)}(t) + C_{ij}^{(2)*}(t) + \sum_k C_{kj}^{(1)*}(t)C_{ki}^{(1)}(t)}_{=0}, \tag{2}$$

where the denoted first and second order terms are required to vanish in order to have unitary evolution, *i.e.*, $\langle j(t)|i(t)\rangle = \delta_{ji}$.

**Density matrix.** The expansion of the time-dependent Kohn–Sham density matrix is

$$\rho_{mn}(t) = \sum_i \langle n|i(t)\rangle f_i \langle i(t)|m\rangle \tag{3}$$

$$= f_n\delta_{nm} + e^{-i(\epsilon_n-\epsilon_m)t}\left[\left(f_n C_{mn}^{(1)*}(t) + f_m C_{nm}^{(1)}(t)\right) + \left(f_n C_{mn}^{(2)*}(t) + f_m C_{nm}^{(2)}(t) + \sum_i f_i C_{ni}^{(1)}(t)C_{mi}^{(1)*}(t)\right)\right] \tag{4}$$

By invoking the conditions from unitary evolution from Eq. (2), the first-order contribution simplifies to

$$\rho_{mn}^{(1)}(t) = e^{-i(\epsilon_n-\epsilon_m)t}(f_m - f_n)C_{nm}^{(1)}(t). \tag{5}$$

Note that in the first order the electron-electron and hole-hole parts of the density matrix are zero: $\rho_{mn}^{(1)}(t) = 0$ for $f_m = f_n$, including the diagonal $\rho_{nn}^{(1)}(t) = 0$.

The leading second-order term of the electron-electron and hole-hole parts is obtained by setting $f_m = f_n$ and using Eqs. (2) and (5) as

$$\rho_{mn}^{(2)}(t) = e^{-i(\epsilon_n-\epsilon_m)t}\left[f_n\left(C_{mn}^{(2)*}(t) + C_{nm}^{(2)}(t)\right) + \sum_i f_i C_{ni}^{(1)}(t)C_{mi}^{(1)*}(t)\right] \tag{6}$$

$$= \sum_i e^{-i(\epsilon_n-\epsilon_m)t}(f_i - f_n)C_{mi}^{(1)*}(t)C_{ni}^{(1)}(t) \tag{7}$$

$$= \sum_i^{f_i\neq f_n} \frac{1}{f_i - f_n}\rho_{in}^{(1)}(t)\rho_{im}^{(1)*}(t) \tag{8}$$

$$= \sum_i^{f_i>f_n} \frac{\rho_{in}^{(1)}(t)}{\sqrt{f_i - f_n}}\frac{\rho_{im}^{(1)*}(t)}{\sqrt{f_i - f_m}} - \sum_i^{f_i<f_n} \frac{\rho_{in}^{(1)}(t)}{\sqrt{f_n - f_i}}\frac{\rho_{im}^{(1)*}(t)}{\sqrt{f_m - f_i}}, \tag{9}$$

the first and second terms of which constitute the electron-electron and hole-hole parts of the density matrix. In particular, the diagonal can be simplified by noting that $|\rho_{in}^{(1)}(t)|^2 = |\rho_{ni}^{(1)}(t)|^2$ to

$$\rho_{nn}^{(2)}(t) = \sum_i^{f_i>f_n}\left|\frac{\rho_{in}^{(1)}(t)}{\sqrt{f_i - f_n}}\right|^2 - \sum_i^{f_i<f_n}\left|\frac{\rho_{ni}^{(1)}(t)}{\sqrt{f_n - f_i}}\right|^2. \tag{10}$$

By defining transition probability

$$P_{ia}(t) = \left|\frac{\delta\rho_{ia}(t)}{\sqrt{f_i - f_a}}\right|^2, \tag{11}$$

Eq. (10) reads

$$\rho^{(2)}_{nn}(t) = \sum_{i}^{f_i>f_n} P_{in}(t) - \sum_{a}^{f_n>f_a} P_{na}(t) = P^{\mathrm{e}}_n(t) - P^{\mathrm{h}}_n(t), \tag{12}$$

where $P^{\mathrm{e}}_n(t)$ and $P^{\mathrm{h}}_n(t)$ corresponds to induced occupations of electrons and holes on state $n$, respectively.

**Energy.** In the Kohn–Sham density-functional theory, the total energy is composed of kinetic, Hartree, and XC contributions, and of the external potential energy (including the potential created by nuclei $v^{\mathrm{ext}}$ and first-order light pulse $v^{\mathrm{pulse}}$),

$$E_{\mathrm{tot}}(t) = T(t) + E_{\mathrm{H}}(t) + E_{\mathrm{xc}}(t) + E_{\mathrm{ext}}(t), \tag{13}$$

respectively. In the basis of KS states, these energy terms are (assuming adiabatic XC kernel)

$$\begin{aligned}
T(t) &= \sum_n f_n \int \mathrm{d}\boldsymbol{r}\psi^*_n(\boldsymbol{r},t)\left(-\frac{1}{2}\nabla^2\right)\psi_n(\boldsymbol{r},t) && (14)\\
&= \sum_{ij} \rho_{ij}(t) t_{ij}, && (15)\\
E_{\mathrm{H}}(t) &= \frac{1}{2}\int \mathrm{d}\boldsymbol{r}\int \mathrm{d}\boldsymbol{r}' n(\boldsymbol{r},t)\frac{1}{|\boldsymbol{r}-\boldsymbol{r}'|}n(\boldsymbol{r}',t) && (16)\\
&= \frac{1}{2}\sum_{ij,kl} \rho_{ij}(t) K^{\mathrm{H}}_{ij,kl}\rho_{kl}(t), && (17)\\
E_{\mathrm{xc}}(t) &= E^{(0)}_{\mathrm{xc}} + \int \mathrm{d}\boldsymbol{r} v_{\mathrm{xc}}(\boldsymbol{r})\delta n(\boldsymbol{r},t) + \frac{1}{2}\int \mathrm{d}\boldsymbol{r}\int \mathrm{d}\boldsymbol{r}'\delta n(\boldsymbol{r},t) K^{\mathrm{xc}}(\boldsymbol{r},\boldsymbol{r}')\delta n(\boldsymbol{r}',t) + \ldots && (18)\\
&= E^{(0)}_{\mathrm{xc}} + \sum_{ij}\delta\rho_{ij}(t) v^{\mathrm{xc}}_{ij} + \frac{1}{2}\sum_{kl}\delta\rho_{ij}(t) K^{\mathrm{xc}}_{ij,kl}\delta\rho_{kl}(t) + \ldots, && (19)
\end{aligned}$$

and

$$\begin{aligned}
E_{\mathrm{ext}}(t) &= \int \mathrm{d}\boldsymbol{r} n(\boldsymbol{r},t)\left[v^{\mathrm{ext}}(\boldsymbol{r}) + v^{\mathrm{pulse}}(\boldsymbol{r},t)\right] && (20)\\
&= \sum_{ij}\rho_{ij}(t)\left[v^{\mathrm{ext}}_{ij} + v^{\mathrm{pulse}}_{ij}(t)\right], && (21)
\end{aligned}$$

where $\rho_{ij}(t) = \rho^{(0)}_{ij} + \rho^{(1)}_{ij}(t) + \rho^{(2)}_{ij}(t) + \ldots$ and $\delta\rho_{ij}(t) = \rho_{ij}(t) - \rho^{(0)}_{ij}$. The perturbation expansions of the energy contributions are

$$\begin{aligned}
T(t) &= T^{(0)} + \sum_{ij}\rho^{(1)}_{ij}(t) t_{ij} && + \sum_{ij}\rho^{(2)}_{ij}(t) t_{ij} && (22)\\
E_{\mathrm{H}}(t) &= E^{(0)}_{\mathrm{H}} + \sum_{ij,kl}\rho^{(1)}_{ij}(t) K^{\mathrm{H}}_{ij,kl}\rho^{(0)}_{kl} && + \sum_{ij,kl}\rho^{(2)}_{ij}(t) K^{\mathrm{H}}_{ij,kl}\rho^{(0)}_{kl} + \frac{1}{2}\sum_{ij,kl}\rho^{(1)}_{ij}(t) K^{\mathrm{H}}_{ij,kl}\rho^{(1)}_{kl}(t) && (23)\\
E_{\mathrm{xc}}(t) &= E^{(0)}_{\mathrm{xc}} + \sum_{ij}\rho^{(1)}_{ij}(t) v^{\mathrm{xc}}_{ij} && + \sum_{ij}\rho^{(2)}_{ij}(t) v^{\mathrm{xc}}_{ij} + \frac{1}{2}\sum_{ij,kl}\rho^{(1)}_{ij}(t) K^{\mathrm{xc}}_{ij,kl}\rho^{(1)}_{kl}(t) && (24)\\
E_{\mathrm{ext}}(t) &= V^{(0)}_{\mathrm{ext}} + \sum_{ij}\rho^{(1)}_{ij}(t) v^{\mathrm{ext}}_{ij} + \rho^{(0)}_{ij} v^{\mathrm{pulse}}_{ij}(t) && + \sum_{ij}\rho^{(2)}_{ij}(t) v^{\mathrm{ext}}_{ij} + \rho^{(1)}_{ij}(t) v^{\mathrm{pulse}}_{ij}(t) && (25)
\end{aligned}$$

(note that here the summations over $ij$ and $kl$ run over all indices, including both the electron-hole and hole-electron spaces and the diagonal).

The first order gives

$$E^{(1)}_{\mathrm{tot}}(t) = \sum_{ij}\rho^{(1)}_{ij}(t)\left[t_{ij} + \sum_{kl} K^{\mathrm{H}}_{ij,kl}\rho^{(0)}_{kl} + v^{\mathrm{xc}}_{ij} + v^{\mathrm{ext}}_{ij}\right] + \rho^{(0)}_{ij} v^{\mathrm{pulse}}_{ij}(t) = \underbrace{\sum_{ij}\rho^{(1)}_{ij}(t) H^{(0)}_{ij}}_{=0} - \mu^{(0)}\mathcal{E}(t), \tag{26}$$

where the first term vanishes as the ground-state Hamiltonian $H_{ij}^{(0)} = \epsilon_i \delta_{ij}$ and $\rho_{ii}^{(1)}(t) = 0$.

The second order gives

$$E_{\rm tot}^{(2)}(t) = \sum_{ij} \rho_{ij}^{(2)}(t) \left[ t_{ij} + \sum_{kl} K_{ij,kl}^{\rm H} \rho_{kl}^{(0)} + v_{ij}^{\rm xc} + v_{ij}^{\rm ext} \right] + \frac{1}{2} \sum_{ij,kl} \rho_{ij}^{(1)}(t) \left( K_{ij,kl}^{\rm H} + K_{ij,kl}^{\rm xc} \right) \rho_{kl}^{(1)}(t) + \sum_{ij} \rho_{ij}^{(1)}(t) v_{ij}^{\rm pulse}(t) \tag{27}$$

$$= \sum_{i} \rho_{ii}^{(2)}(t) \epsilon_i + \frac{1}{2} \sum_{ij,kl} \rho_{ij}^{(1)}(t) K_{ij,kl}^{\rm Hxc} \rho_{kl}^{(1)}(t) - \mu^{(1)}(t) \mathcal{E}(t). \tag{28}$$

By using Eq. (12) and assuming real-valued ground-state KS wave functions and frequency-independent XC kernel, simplifying the Hartree-XC term, [1] Eq. (28) can be written as a sum over electron-hole space only

$$E_{\rm tot}^{(2)}(t) = \sum_{ia}^{f_i > f_a} \underbrace{\left[ \omega_{ia} P_{ia}(t) + \underbrace{\frac{1}{2} \cdot 2\Re\rho_{ia}^{(1)}(t) \sum_{jb}^{f_j > f_b} K_{ia,jb}^{\rm Hxc} 2\Re\rho_{jb}^{(1)}(t)}_{=E_{ia}^{\rm C}(t)} \right]}_{=E_{ia}(t)} - \mu^{(1)}(t) \mathcal{E}(t), \tag{29}$$

where the Hartree-XC term is used to estimate the Coulomb energy $E_{ia}^{\rm C}(t)$. In RPA, the XC is neglected and $K^{\rm Hxc}$ is replaced by the Hartree kernel $K^{\rm H}(\boldsymbol{r}, \boldsymbol{r}') = |\boldsymbol{r} - \boldsymbol{r}'|^{-1}$.

By collecting all the terms, the energy up to the second order is

$$E_{\rm tot}(t) = E_{\rm tot}^{(0)} + \sum_{ia}^{f_i > f_a} E_{ia}(t) - \underbrace{\left[ \mu^{(0)} + \mu^{(1)}(t) \right] \mathcal{E}(t)}_{=\mu(t)\mathcal{E}(t) = -E_{\rm pulse}(t)}. \tag{30}$$

**Supplementary Note S2: Energy in terms of real and imaginary parts of density matrix.**

The real and imaginary parts of the time-dependent density matrix have a well-defined connection [Eq. (4.25) of Ref. 1]. By assuming real-valued ground-state wave functions and a frequency-independent XC kernel, the connection can be expressed in electron-hole space in the time domain as

$$\begin{cases} \Re\delta\dot{\rho}_{ia}(t) = -\omega_{ia} \Im\delta\rho_{ia}(t) \\ \Im\delta\dot{\rho}_{ia}(t) = \omega_{ia} \Re\delta\rho_{ia}(t) + (f_i - f_a) \sum_{jb}^{f_j > f_b} K_{ia,jb}^{\rm Hxc} 2\Re\delta\rho_{jb}(t) + (f_i - f_a) v_{ia}^{\rm pulse}(t) \end{cases}, \tag{31}$$

where dots denote time derivatives. By defining the auxiliary quantities

$$q_{ia}(t) = \frac{2\Re\delta\rho_{ia}(t)}{\sqrt{2(f_i - f_a)}}, \quad p_{ia}(t) = -\frac{2\Im\delta\rho_{ia}(t)}{\sqrt{2(f_i - f_a)}}, \tag{32}$$

$$K_{ia,jb} = \sqrt{2(f_i - f_a)} K_{ia,jb}^{\rm Hxc} \sqrt{2(f_j - f_b)}, \quad \text{and} \quad v_{ia}(t) = \sqrt{2(f_i - f_a)} v_{ia}^{\rm pulse}(t), \tag{33}$$

Eq. (31) can be written in convenient form as

$$\begin{cases} \dot{q}_{ia}(t) = \omega_{ia} p_{ia}(t) \\ \dot{p}_{ia}(t) = -\omega_{ia} q_{ia}(t) - \sum_{jb} K_{ia,jb} q_{jb}(t) - v_{ia}(t) \end{cases}. \tag{34}$$

These equations are identical to the equations of motion of a collection of coupled classical harmonic oscillators when $q_{ia}(t)$ and $p_{ia}(t)$ are identified as position and momentum coordinates. In this notation, the electron-hole decomposition of energy of Eq. (29) is

$$E_{ia}(t) = \frac{1}{2} \left[ \omega_{ia} p_{ia}^2(t) + \omega_{ia} q_{ia}^2(t) + q_{ia}(t) \sum_{jb} K_{ia,jb} q_{jb}(t) \right], \tag{35}$$

and the Coulomb energy contribution from Eq. (29) is

$$E^{\mathrm{C}}_{ia}(t) = \frac{1}{2} q_{ia}(t) \sum_{jb} K_{ia,jb} q_{jb}(t). \tag{36}$$

**Supplementary Note S3: Rate of energy change.**

By evaluating the time differential of Eq. (35) and using the equations of motion of Eq. (34), the rate of change of the electronic energy is obtained as

$$\dot{E}_{ia}(t) = \underbrace{\frac{1}{2}\left[ q_{ia}(t) \sum_{jb} K_{ia,jb} \dot{q}_{jb}(t) - \dot{q}_{ia}(t) \sum_{jb} K_{ia,jb} q_{jb}(t) \right]}_{\text{interaction}} \underbrace{- v_{ia}(t) \dot{q}_{ia}(t)}_{\text{photoabsorption}}, \tag{37}$$

where the terms related to the interaction between electron-hole transitions and to photoabsorption have been identified. When summing over all transitions, the interaction term vanishes due to the symmetry of the $K_{ia,jb}$ matrix (see note above), and the total rate of change is

$$\Delta \dot{E}(t) = \sum_{ia} \dot{E}_{ia}(t) = -\sum_{ia} \dot{q}_{ia}(t) v_{ia}(t) = -\sum_{ia}^{f_i > f_a} 2 \Re \delta \dot{\rho}_{ia}(t) v^{\text{pulse}}_{ia}(t) = \delta \dot{\mu}(t) \mathcal{E}(t), \tag{38}$$

where $\delta\mu(t)$ is the induced dipole moment.

**Supplementary Note S4: Practical evaluation of energy and its rate of change.**

In practical calculations, $E_{ia}(t)$, $E^{\mathrm{C}}_{ia}(t)$, and $\dot{E}_{ia}(t)$ can be evaluated without explicit knowledge of the $K_{ia,jb}$ matrix. This is done by employing Eq. (34), resulting in the following practical forms of Eqs. (35), (36), and (37):

$$E_{ia}(t) = \frac{1}{2}\left[ p_{ia}(t) \dot{q}_{ia}(t) - q_{ia}(t) \dot{p}_{ia}(t) - v_{ia}(t) q_{ia}(t) \right], \tag{39}$$

$$E^{\mathrm{C}}_{ia}(t) = -\frac{1}{2}\left[ \omega_{ia} q^2_{ia}(t) + q_{ia}(t) \dot{p}_{ia}(t) + v_{ia}(t) q_{ia}(t) \right], \tag{40}$$

and

$$\dot{E}_{ia}(t) = \underbrace{\frac{1}{2}\left[ p_{ia}(t) \ddot{q}_{ia}(t) - q_{ia}(t) \ddot{p}_{ia}(t) + v_{ia}(t) \dot{q}_{ia}(t) - \dot{v}_{ia}(t) q_{ia}(t) \right]}_{\text{interaction}} \underbrace{- v_{ia}(t) \dot{q}_{ia}(t)}_{\text{photoabsorption}}, \tag{41}$$

respectively.

# Supplementary References


[1] M. E. Casida, *Time-Dependent Density Functional Response Theory for Molecules,* in *Recent Advances in Density Functional Methods, Part I*, edited by D. P. Chong (World Scientific, Singapore, 1995), p. 155. doi:10.1142/9789812830586_0005.
